# Supplementary material for: Straightening Out the Straight-Through Estimator: Overcoming Optimization Challenges in Vector Quantized Networks
Source: arXiv:2305.08842 source file (2023-05-15)
Supplement: Supplementary file 1 [file 7_appendix.tex]

\newpage
\section{Appendix}
\subsection{Additional training details}
\label{app:details}
All models were trained using PyTorch on RTX2080Ti. We use a batch size $128$ for all experiments.
We use standard ResNet-ImageNet training procedure: SGD optimizer with learning rate $0.1$, momentum $0.9$, weight-decay $10^{-4}$, and Inception data augmentation~\cite{szegedy2015going}. We train for $120$ epochs and scale the learning rate by a factor of $\frac{1}{10}$ at epoch $80$. 
HVQNs with $\mathsf{4VQ}$ layers requires approximately $1.5-2.0\times$ more training time. As the numerical precision of distance function is not important, we compute it in half precision. We compute the distance matrix via divide-and-conquer and compute the top-k reduction on-the-fly; hence our implementation requires very little memory overhead. We found this to work better than using nearest-neighbor libraries (\eg FAISS) and reduction libraries (\eg pykeops).

The full training code and the trained weights will be released upon acceptance.

\newpage
\subsection{Distribution}
\label{app:dist}
In~\sect{sec:quantization}, we demonstrated that the empirical divergence between the codebook and the embedding is large when a wrong distribution is assumed. Hence to reduce the quantization error one requires a priori knowledge of what the embedding distribution is going to be. While there is no one-size-fits-all distribution, we demonstrate that a data-dependent distribution can better reduce the divergence.

\begin{figure}[h!]
    \centering
    \begin{subfigure}[b]{\textwidth}
            \centering
            \caption{$\bz_e = \texttt{tanh}(\texttt{conv}(\bx))\quad \lvert \quad \bx \sim \mathcal{N}(0, 1)$}
            \includegraphics[width=\textwidth]{./images/mmd_conv_tanh_normal_data.pdf}
    \end{subfigure}\\
    \begin{subfigure}[b]{\textwidth}
            \centering
            \caption{$\bz_e = \texttt{relu}(\texttt{bn}(\texttt{conv}(\bx))) + \bx\quad \lvert \quad\bx \sim \mathcal{N}(0, 1)$}
            \includegraphics[width=\textwidth]{./images/mmd_residual_normal_data.pdf}
    \end{subfigure}\\
    \begin{subfigure}[b]{\textwidth}
            \centering
            \caption{$\bz_e = \texttt{tanh}(\texttt{bn}(\texttt{conv}(\bx))) + \bx\quad \lvert \quad\bx \sim \mathcal{N}(0, 1)$}
            \includegraphics[width=\textwidth]{./images/mmd_residual_tanh_normal_data.pdf}
    \end{subfigure}\\
    
    \begin{subfigure}[b]{\textwidth}
            \centering
            \caption{$\bz_e = \texttt{tanh}(\texttt{conv}(\bx))\quad \lvert \quad\bx \sim \mathcal{U}(-2, 2)$}
            \includegraphics[width=\textwidth]{./images/mmd_conv_tanh_uniform_data.pdf}
    \end{subfigure}\\
    \begin{subfigure}[b]{\textwidth}
            \centering
            \caption{$\bz_e = \texttt{relu}(\texttt{bn}(\texttt{conv}(\bx))) + \bx\quad \lvert \quad\bx \sim \mathcal{U}(-2, 2)$}
            \includegraphics[width=\textwidth]{./images/mmd_residual_uniform_data.pdf}
    \end{subfigure}\\
    \begin{subfigure}[b]{\textwidth}
            \centering
            \caption{$\bz_e = \texttt{tanh}(\texttt{bn}(\texttt{conv}(\bx))) + \bx\quad \lvert \quad\bx \sim \mathcal{U}(-2, 2)$}
            \includegraphics[width=\textwidth]{./images/mmd_residual_tanh_uniform_data.pdf}
    \end{subfigure}
    \caption{Additional examples of the empirical divergence between the embedding $\bz_e$ and the quantized embedding $\bz_q$.}
\end{figure}

\newpage

\subsection{Quantization error}
\label{app:training}
In~\fig{fig:training}, we show the training dynamics of various model configurations. The figure highlights how each component of the proposed method affects the dynamics of the training. 

\begin{figure}[h!]
\centering
  \includegraphics[width=1.0\textwidth]{./images/training_dynamics.pdf}
  \caption{\small Training dynamics of various model configurations. On the left we show the training accuracy, testing accuracy and the commitment loss. On the right we show the gradient approximation error. We provide a zoomed in view of gradient error without euclidean VQ for clarity.}
  \label{fig:training}
\end{figure}

\newpage
\subsection{Additional code collages}
\label{app:more_collage}

\begin{figure}[h!]
\centering
  \includegraphics[width=1.0\textwidth]{./images/l3_g0_c115.png}\\
  \includegraphics[width=1.0\textwidth]{./images/l3_g0_c167.png}\\
  \includegraphics[width=1.0\textwidth]{./images/l3_g0_c182.png}\\
\end{figure}

\begin{figure}[h!]
\centering
  \includegraphics[width=1.0\textwidth]{./images/l3_g1_c28.png}\\
  \includegraphics[width=1.0\textwidth]{./images/l3_g1_c45.png}\\
  \includegraphics[width=1.0\textwidth]{./images/l3_g1_c221.png}\\
  \caption{\small Additional code collage.}
  \label{fig:training}
\end{figure}

\begin{figure}[h!]
\centering
  \includegraphics[width=1.0\textwidth]{./images/l3_g2_c53.png}\\
  \includegraphics[width=1.0\textwidth]{./images/l3_g2_c60.png}\\
  \includegraphics[width=1.0\textwidth]{./images/l3_g2_c74.png}\\
  \caption{\small Additional code collage.}
  \label{fig:training}
\end{figure}

\begin{figure}[h!]
\centering
  \includegraphics[width=1.0\textwidth]{./images/l3_g3_c221.png}\\
  \includegraphics[width=1.0\textwidth]{./images/l3_g3_c279.png}\\
  \includegraphics[width=1.0\textwidth]{./images/l3_g3_c351.png}\\
  \caption{\small Additional code collage.}
  \label{fig:training}
\end{figure}
